# Supplementary material for: Simplex Random Features
Source: arXiv:2301.13856 source file (2023-10-07)
Supplement: Supplementary file 1 [file main_appendix.tex]

\section{Supplementary proofs and discussion}\label{proofs_app}
In this appendix we provide further discussion and proofs of results stated in the main text.

\subsection{Analytic expressions for the orthogonality gap with RFFs and PRFs} \label{app:sec1}
In this section, we provide proofs for the explicit formulae on the orthogonality gap with RFFs and PRFs. The proofs of the technical lemmas used here are provided in the following sections. 
\input{section_1}
\input{proofs_appendix.tex}
\section{Experimental details}\label{exp_appendix}
\input{exp_appendix.tex}
\input{extra_appendix.tex}
